# Supplementary material for: Modeling the Equilibrium Vacancy Concentration in Multi-Principal Element Alloys from First-Principles
Source: arXiv:2509.21944 source file (2025-09-26)
Supplement: Supplementary file 1 [file Si.pdf]

# Supplementary Material: Modeling the Equilibrium Vacancy Concentration in Multi-Principal Element Alloys from First-Principles

Damien K. J. Lee,<sup>1</sup> Yann L. Müller,<sup>1</sup> and Anirudh Raju Natarajan<sup>1,2</sup>

<sup>1</sup>*Laboratory of materials design and simulation (MADES),  
Institute of Materials, École Polytechnique Fédérale de Lausanne*  
<sup>2</sup>*National Centre for Computational Design and Discovery of Novel  
Materials (MARVEL), École Polytechnique Fédérale de Lausanne*

## S1 Pseudopotentials used in DFT calculations

| Element | POTCAR          |
|---------|-----------------|
| Ti      | Ti_sv 26Sep2005 |
| Zr      | Zr_sv 04Jan2005 |
| Hf      | Hf_pv 06Sep2000 |
| V       | V_sv 02Aug2007  |
| Nb      | Nb_sv 25May2007 |
| Ta      | Ta_pv 07Sep2000 |
| Cr      | Cr_pv 02Aug2007 |
| Mo      | Mo_sv 02Feb2006 |
| W       | W_sv 04Sep2015  |

TABLE S1: Pseudopotentials used in DFT calculations

## S2 Trade-off between model complexity and evaluation speed

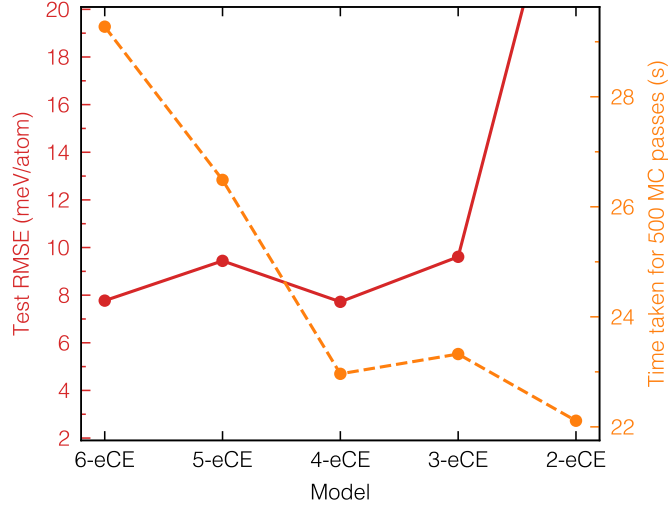

FIG. S1: Comparisons between  $k$ -eCE models where  $k$  represent the embedding dimension of the model. The red curve represents the RMSE of the test set of the model while the orange curve represents the time taken to evaluate 500 MC passes on a  $10 \times 10 \times 10$  supercell of the conventional BCC cell.

### S3 Convex hulls of binary subsystems predicted by DFT and eCE

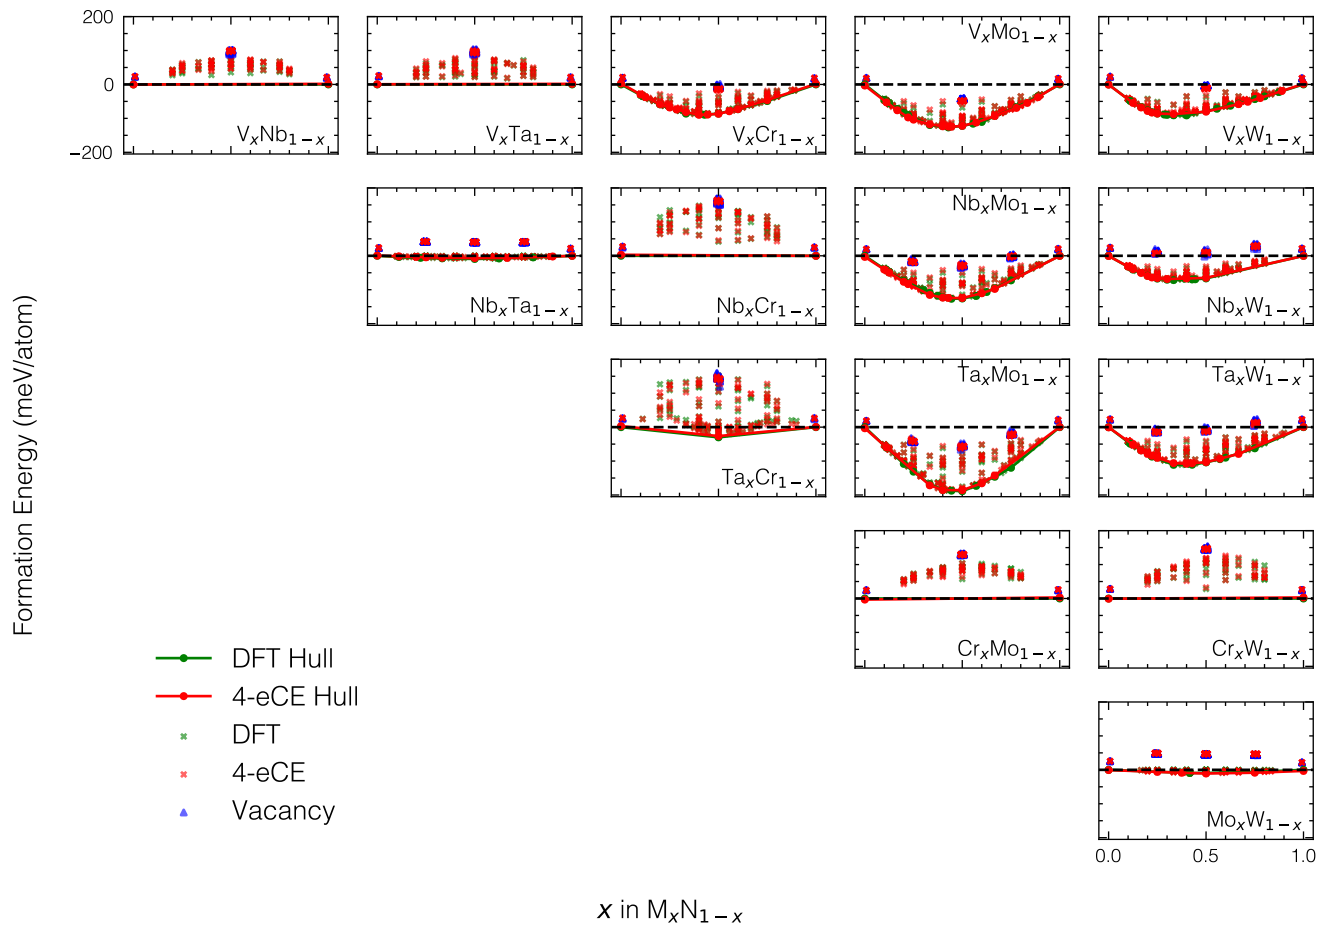

FIG. S2: Convex hulls of the binary systems of Group 5 and 6 elements.

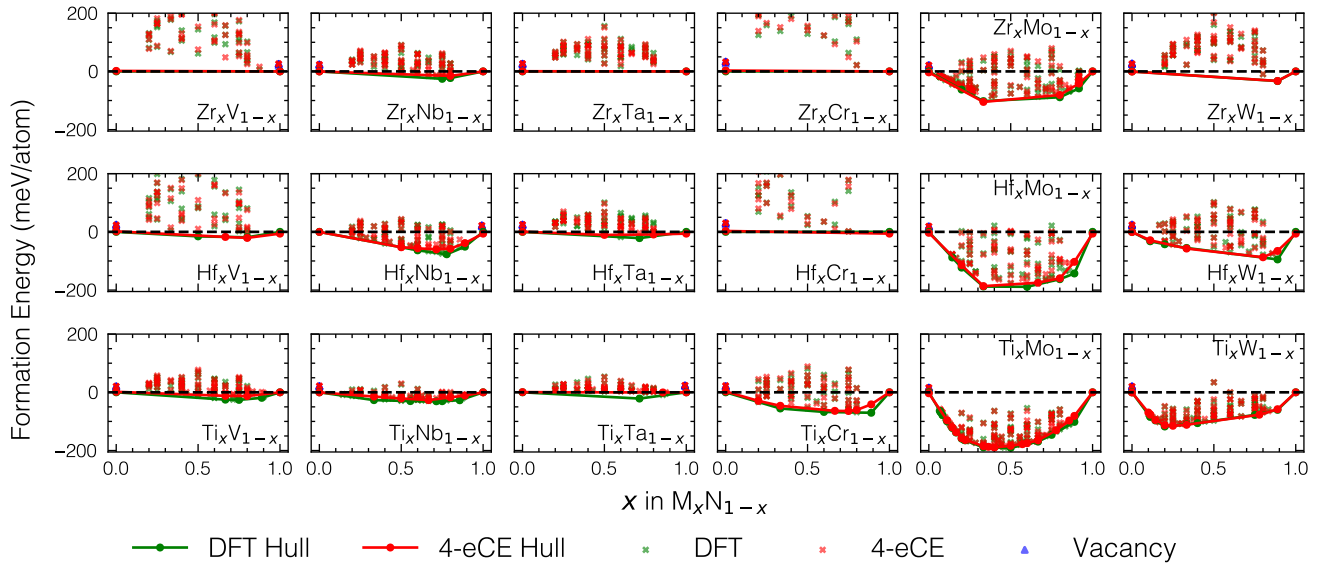

FIG. S3: Convex hulls of the binary systems of Group 4 elements alloyed with Group 5 and 6 elements.

#### S4 Parity plot of model prediction and DFT calculations

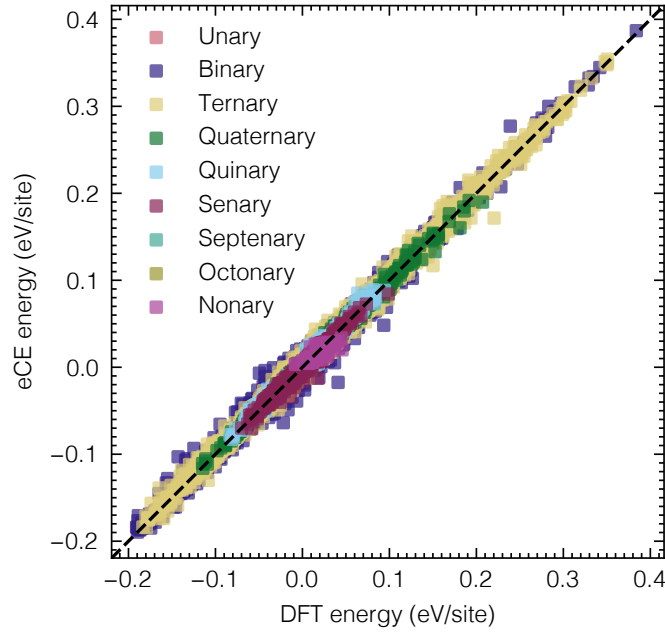

FIG. S4: Parity plot of formation energies predicted using the 4-eCE model and DFT calculations. Each point is color-coded by the alloy's chemical complexity.

## S5 Effect of solute size on vacancy binding energy

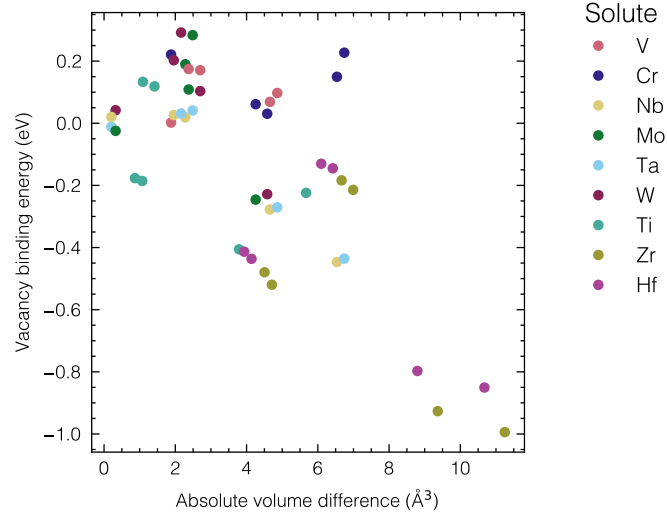

FIG. S5: Vacancy binding energy as a function of the metallic volume difference between solute and solvent atoms. The vacancy binding energy is defined as the energy difference between a configuration with the solute in the first nearest-neighbor shell of the vacancy and one where the solute is placed at the furthest distance from the vacancy.

## S6 Substitution of VNbTaCrMoW with Zr

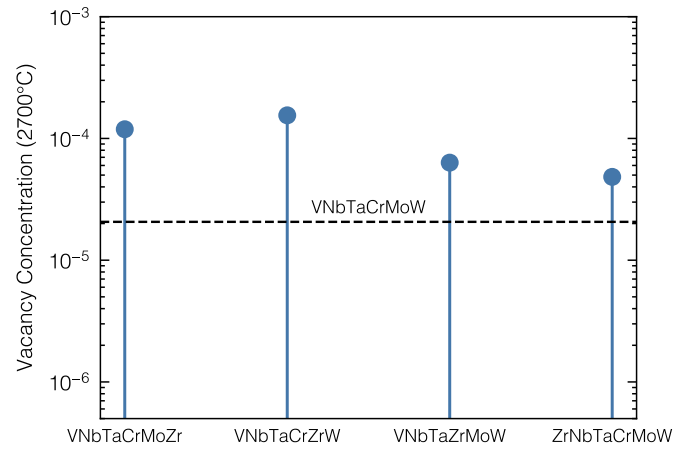

FIG. S6: Vacancy concentration at 2700°C for each element in VNbTaCrMoW substituted with Zr. Alloys which are found to be unstable at 2700°C are not shown in the plot.

# S7 Vacancy-solute binding energies for Hf, Zr, Mo, Nb, Ti

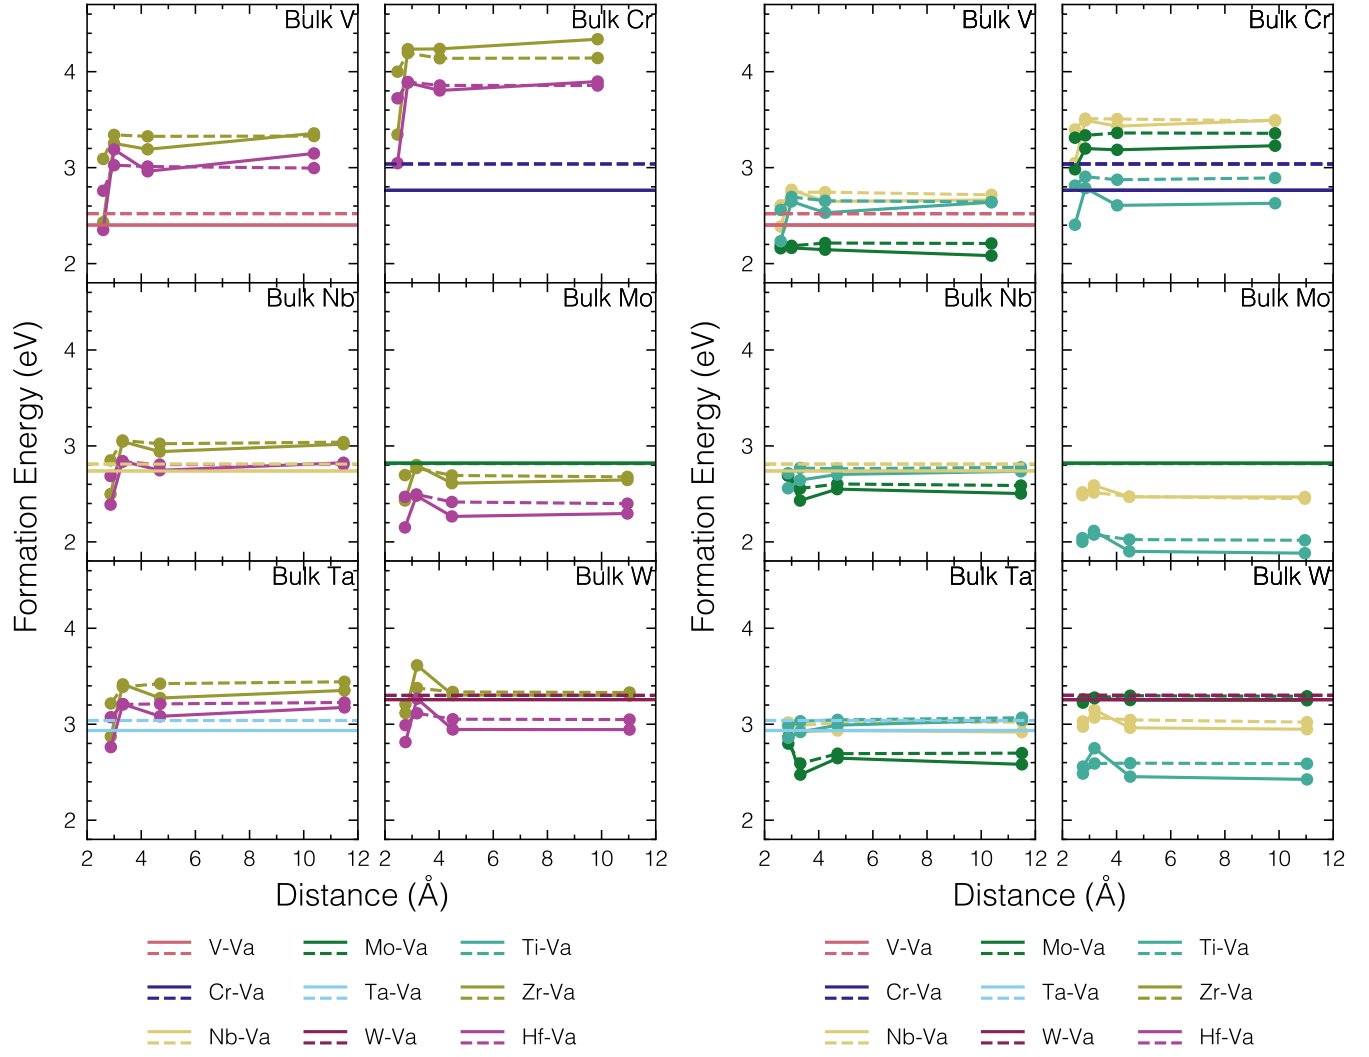

FIG. S7: Formation energies of vacancy-solute structures for Hf, Zr (left), Nb, Mo, Ti (right) solutes in a bulk system. Values shown are identical to fig. 3 but are separated for clarity.

## S8 Heat capacities obtained from Monte Carlo

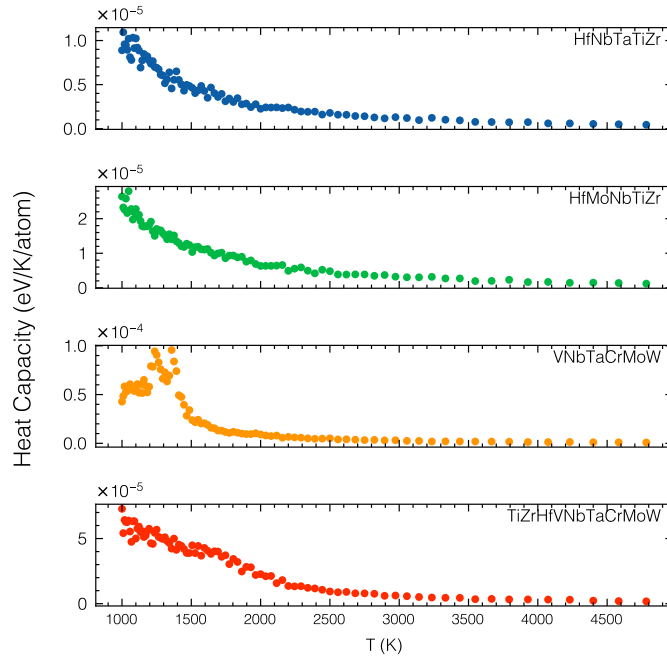

FIG. S8: Heat capacities of the 4 different alloys studied in fig. 5, calculated as a function of temperature during the cooling run.

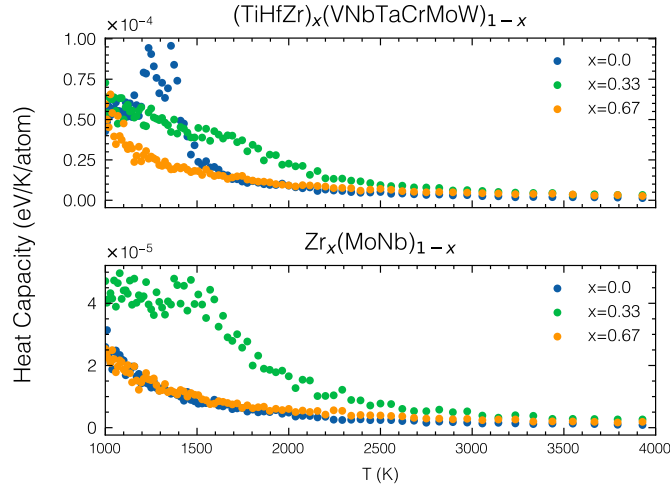

FIG. S9: Heat capacities of the alloys studied in Figure 7, where  $x=[0, 0.33, 0.67]$ , as calculated as a function of temperature during the cooling run.

## S9 Variation in vacancy concentration with the species being swapped

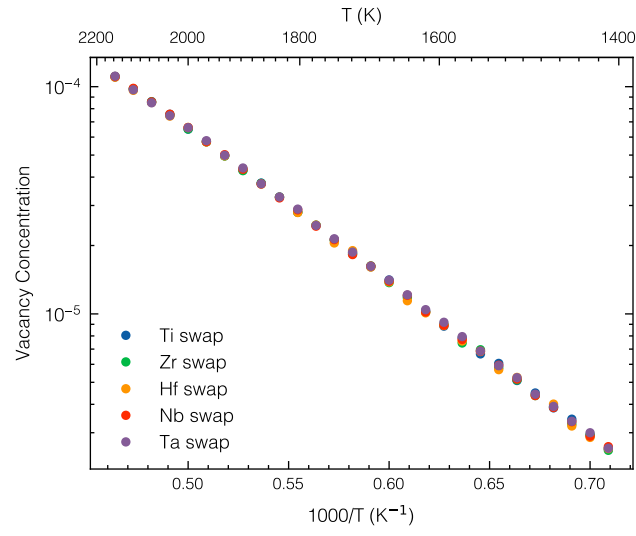

FIG. S10: Vacancy concentration calculated by performing vacancy swaps with the different chemical species in the HfNbTaTiZr alloy.

# S10 Exchange chemical potentials calculated using the Widom substitution method

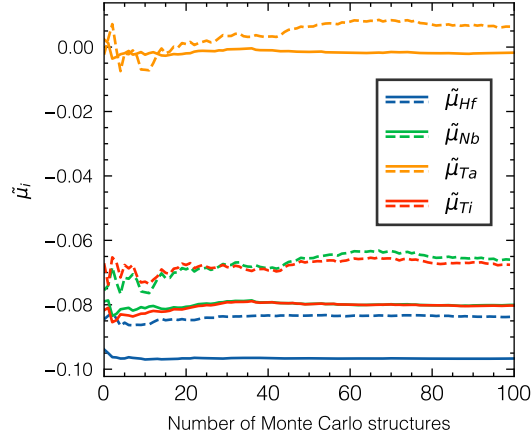

FIG. S11: Exchange chemical potentials calculated using the Widom substitution method, as a function of the number of structures drawn from a MC simulation. The solid line and dashed line indicate the substitution was performed in a large cell (2000 atoms) and a small cell (128 atoms) respectively. The exchange chemical potentials are defined as  $\tilde{\mu}_i = \mu_i - \mu_{Zr}$  in the HfNbTaTiZr alloy.
